# Supplementary material for: Mining Architectural Information: A Systematic Mapping Study
Source: arXiv:2212.13179 source file (2024-04-04)
Supplement: Supplementary file 1 [file appendix.tex]

% \section*{Appendix} \label{appendix}

% \subsection*{Appendix A. Selected Studies}\label{SlectedStudies}
% \noindent{[S1]}	M. Soliman, M. Galster, P. Avgeriou, An exploratory study on architectural knowledge in issue tracking systems, in: Proceedings of the 15th European Conference on Software Architecture (ECSA), 2021, pp. 117–133 \\
% {[S2]}	M. Soliman, M. Wiese, Y. Li, M. Riebisch, P. Avgeriou, Exploring web search engines to find architectural knowledge, in: Proceedings of the 18th IEEE International Conference on Software Architecture (ICSA), 2021, pp. 162–172 \\
% {[S3]}	M. Soliman, A. R. Salama, M. Galster, O. Zimmermann, M. Riebisch, Improving the search for architecture knowledge in online developer communities, in: Proceedings of the 15th IEEE International Conference on Software Architecture (ICSA), 2018, pp. 186–195 \\	
% {[S4]}	M. Soliman, M. Galster, A. R. Salama, M. Riebisch, Architectural knowledge for technology decisions in developer communities: An exploratory study with Stack Overflow, in: Proceedings of the 13th Working IEEE/IFIP Conference on Software Architecture (WICSA), 2016, pp. 128–133 \\
% {[S5]}	F. Tian, F. Lu, P. Liang, M. A. Babar, Automatic identification of architecture smell discussions from Stack Overflow, In: Proceedings of the 32nd International Conference on Software Engineering and Knowledge Engineering (SEKE), 2020, pp. 451–456 \\
% {[S6]}	T. Bi, P. Liang, A. Tang, X. Xia, Mining architecture tactics and quality attributes knowledge in Stack Overflow, Journal of Systems and Software 180 (2021) 111005 \\
% {[S7]}	I. Malavolta, K. Chinnappan, S. Swanborn, G. A. Lewis, P. Lago, Mining the ROS ecosystem for green architectural tactics in robotics and an empirical evaluation. in: Proceedings of the 18th International Working Conference on Mining Software Repositories (MSR), 2021, pp. 300-311 \\	
% {[S8]} I. Malavolta, G. A. Lewis, B. Schmerl, P. Lago, D. Garlan, Mining guidelines for architecting robotics software, Journal of Systems and Software 178 (2021) 110969 \\
% {[S9]}	K. Chinnappan, I. Malavolta, G. A. Lewis, M. Albonico, P. Lago, Architectural tactics for energy-aware robotics software: A preliminary study, in: Proceedings of the 15th European Conference on Software Architecture (ECSA), 2021, pp. 164–171 \\
% {[S10]}	M. Borg, I. Lennerstad, R. Ros, E. Bjarnason, On using active learning and self-training when mining performance discussions on stack overflow, in: Proceedings of the 21st International Conference on Evaluation and Assessment in Software Engineering (EASE), 2017, pp. 308–313 \\
% {[S11]}	T. Bi, W. Ding, P. Liang, A. Tang, Architecture information communication in two OSS projects: The why, who, when, and what, Journal of Systems and Software 181 (2021) 111035 \\
% {[S12]} S. Nadi, T. Berger, C. K\"{a}stner, K. Czarnecki, Mining configuration constraints: Static analyses and empirical results, in: Proceedings of the 36th International Conference on Software Engineering (ICSE), 2014, pp. 140–151 \\
% {[S13]}	M. J. Mujhid, J. C. Santos, R. Gopalakrishnan, M. Mirakhorli, A search engine for finding and reusing architecturally significant code, Journal of Systems and Software 130 (2017) 81–93 \\
% {[S14]} A. Zalewski, K. Borowa, K. Lisocki, Supporting architectural decision-making with data retrieved from online communities, in: Proceedings of the 16th International Conference on Dependability and Complex Systems (DepCoS-RELCOMEX), 2021, pp. 496–509 \\
% {[S15]}	I. Gorton, R. Xu, Y. Yang, H. Liu, G. Zheng, Experiments in curation: Towards machine-assisted construction of software architecture knowledge bases, in: Proceedings of the 14th IEEE International Conference on Software Architecture (ICSA), 2017, pp. 79–88 \\
% {[S16]}	G. Borrego, A. L. Mor\'{a}n, R. R. Palacio, A. Vizca\'{i}no, F. O. Garc\'{i}a, Towards a reduction in architectural knowledge vaporization during agile global software development, Information and Software Technology 112 (2019) 68–82 \\
% {[S17]}	G. Viviani, M. Famelis, X. Xia, C. Janik-Jones, G. C. Murphy, Locating latent design information in developer discussions: A study on pull requests, IEEE Transactions on Software Engineering 47 (7) (2019) 1402–1413 \\
% {[S18]}	J. S. v. d. Ven, J. Bosch, Making the right decision: supporting architects with design decision data, in: Proceedings of the 7th European Conference on Software Architecture (ECSA), 2013, pp. 176–183 \\
% {[S19]}	M. Bhat, C. Tinnes, K. Shumaiev, A. Biesdorf, U. Hohenstein, F. Matthes, Adex: A tool for automatic curation of design decision knowledge for architectural decision recommendations, in: Proceedings of the 6th IEEE International Conference on Software Architecture Companion (ICSA-C), 2019, pp. 158–161 \\
% {[S20]}	S. Karthik, N. Medvidovic, Automatic detection of latent software component relationships from online Q\&A sites, in: Proceedings of the 7th IEEE/ACM International Workshop on Realizing Artificial Intelligence Synergies in Software Engineering (RAISE), 2019, pp. 15–21 \\
% {[S21]}	M. Mirakhorli, P. M\"{a}der, J. Cleland-Huang, Variability points and design pattern usage in architecture tactics, in: Proceedings of the 20th ACM SIGSOFT International Symposium on the Foundations of Software Engineering (FSE), 2012, pp. 1–11 \\
% {[S22]}	M. Bhat, K. Shumaiev, A. Biesdorf, U. Hohenstein, F. Matthes, Automatic extraction of design decisions from issue management systems: a machine learning based approach, in: Proceedings of the 11th European Conference on Software Architecture (ECSA), 2017, pp. 138–154 \\
% {[S23]}	Aman-ul-haq, M. A. Babar, Tool support for automating architectural knowledge extraction, in: Proceeding on the 4th Workshop on SHAring and Reusing architectural Knowledge (SHARK), 2009, pp. 49–56 \\
% {[S24]}	C. L\'{o}pez, V. Codocedo, H. Astudillo, L. M. Cysneiros, Bridging the gap between software architecture rationale formalisms and actual architecture documents: An ontology-driven approach, Science of Computer Programming 77 (1) (2012) 66–80 \\
% {[S25]}	B. Rogers, Y. Qiao, J. Gung, T. Mathur, J. E. Burge, Using text mining techniques to extract rationale from existing documentation, in: Proceedings of the 9th International Conference on Design Computing and Cognition (DCC), 2014, pp. 457–474 \\
% {[S26]}	G. M\'{a}rquez, M. M. Villegas, H. Astudillo, An empirical study of scalability frameworks in open source microservices-based systems, in: Proceedings of the 37th IEEE International Conference of the Chilean Computer Science Society (SCCC), 2018, pp. 1–8 \\
% {[S27]}	R. Gopalakrishnan, P. Sharma, M. Mirakhorli, M. Galster, Can latent topics in source code predict missing architectural tactics?, in: Proceedings of the 39th IEEE/ACM International Conference on Software Engineering (ICSE), 2017, pp. 15–26 \\
% {[S28]}	A. M. Figueiredo, J. C. Dos Reis, M. A. Rodrigues, Improving access to software architecture knowledge an ontology-based search approach, International Journal Multimedia and Image Processing 2 (1/2) (2012) 124–149 \\
% {[S29]}	J. Soldani, G. Muntoni, D. Neri, A. Brogi, The $\mu$TOSCA toolchain-Mining, analyzing, and refactoring microservice‐based architectures, Software: Practice and Experience 51 (7) (2021) 1591–1621 \\
% {[S30]}	N. Ghorbani, J. Garcia, S. Malek, Detection and repair of architectural inconsistencies in java, in: Proceedings of the 41st IEEE/ACM  International Conference on Software Engineering (ICSE), 2019, pp. 560–571 \\
% {[S31]}	P. Velasco-Elizondo, R. Mar\'{i}ın-Pi\H{n}a, S. Vazquez-Reyes, A. Mora-Soto, J. Mejia, Knowledge representation and information extraction for analysing architectural patterns, Science of Computer Programming 121 (2016) 176–189 \\
% {[S32]}	M. L. Rold\'{a}an, S. Gonnet, H. Leone, An ontology-based approach for sharing, integrating, and retrieving architectural knowledge, Electronic Notes in Theoretical Computer Science 339 (2018) 43-62 \\
% {[S33]}	L. Lee, P. Kruchten, Customizing the capture of software architectural design decisions, in: Proceedings of the 21st Annual Canadian Conference on Electrical and Computer Engineering (CCECE), 2008, pp. 693–698. \\
% {[S34]}	C. Maffort, M. T. Valente, R. Terra, M. Bigonha, N. Anquetil, A. Hora, Mining architectural violations from version history, Empirical Software Engineering, 21 (3) (2016) 854–895 \\
% {[S35]}	A. Shahbazian, D. Nam, N. Medvidovic, Toward predicting architectural significance of implementation issues, in: Proceedings of the 15th International Working Conference on Mining Software Repositories (MSR), 2018, pp. 215–219 \\
% {[S36]}	R. Talwadker, D. Aggarwal, Popcon: Mining popular software configurations from community, in: Proceedings of the 13th ACM/IEEE International Symposium on Empirical Software Engineering and Measurement (ESEM), 2019, pp. 1-6 \\
% {[S37]}	R. Kazman, Y. Cai, R. Mo, Q. Feng, L. Xiao, S. Haziyev, V. Fedak, A. Shapochka, A case study in locating the architectural roots of technical debt, in: Proceedings of the 37th IEEE International Conference on Software Engineering (ICSE), 2015, pp. 179-188 \\
% {[S38]}	M. X. Liu, J. Hsieh, N. Hahn, A. Zhou, E. Deng, S. Burley, C. Taylor, A. Kittur, B. A. Myers, Unakite: Scaffolding developers’ decision-making using the web, in: Proceedings of the 32nd Annual ACM Symposium on User Interface Software and Technology (UIST), 2019, pp. 67-80 \\
% {[S39]}	G. Granchelli, M. Cardarelli, P. Di Francesco, I. Malavolta, L. Iovino, A. Di Salle, Towards recovering the software architecture of microservice-based systems, in: Proceedings of the 14th IEEE International Conference on Software Architecture Workshops (ICSAW), 2017, pp. 46–53 \\
% {[S40]}	A. K. Mondal, B. Roy, S. S. Nath, K. A. Schneider, Archinet: A concept-token based approach for determining architectural change categories, In: Proceedings of the 33rd International Conference on Software Engineering and Knowledge Engineering (SEKE), 2021, pp. 7-14 \\
% {[S41]}	J. Garcia, D. Popescu, C. Mattmann, N. Medvidovic, and Y. Cai, Enhancing architectural recovery using concerns, In Preceding of the 16th IEEE International Conference on Automated Software Engineering (ASE), 2011, pp. 552-555  \\
% {[S42]}	F. Gilson, M. Galster, F. Georis, Extracting quality attributes from user stories for early architecture decision making, in: Proceedings of the 16th IEEE International Conference on Software Architecture Companion (ICSA-C), 2019, pp. 129–136 \\
% {[S43]}	A. Casamayor, D. Godoy, M. Campo, Functional grouping of natural language requirements for assistance in architectural software design, Knowledge-Based Systems 30 (2012) 78-86 \\
% {[S44]} K. A. de Graaf, A. Tang, P. Liang, A. Khalili, Querying software architecture knowledge as linked open data, in: Proceedings of the 14th IEEE International Conference on Software Architecture Workshops (ICSAW), 2017, pp. 272–277 \\
% {[S45]}	X. Lian, W. Liu, L. Zhang, Assisting engineers extracting requirements on components from domain documents, Information and Software Technology 118 (2020) 106196 \\
% {[S46]}	P. Behnamghader, D. M. Le, J. Garcia, D. Link, A. Shahbazian, N. Medvidovic, A large-scale study of architectural evolution in open-source software systems, Empirical Software Engineering, 22 (3) (2017) 1146–1193 \\
% {[S47]}	A. Shahbazian, Y. K. Lee, D. Le, Y. Brun, N. Medvidovic, Recovering architectural design decisions, in: Proceedings of the 15th IEEE International Conference on Software Architecture (ICSA), 2018, pp. 95–104 \\
% {[S48]}	A. Mahadi, K. Tongay, N. A. Ernst, Cross-dataset design discussion mining, in: Proceedings of the 27th International Conference on Software Analysis, Evolution and Reengineering (SANER), 2020, pp. 149–160 \\
% {[S49]}	A. Shakiba, R. Green, R. Dyer, ArCode: Facilitating the Use of Application Frameworks to Implement Tactics and Patterns, in: Proceedings of the 18th IEEE International Conference on Software Architecture (ICSA), 2021, pp. 138-149 \\
% {[S50]}	M. T. Su, J. Hosking, J. Grundy, Capturing architecture documentation navigation trails for content chunking and sharing, in: Proceedings of the 9th Working IEEE/IFIP Conference on Software Architecture (WICSA), 2011, pp. 256–259 \\
% {[S51]}	M. Chaabane, I. B. Rodriguez, K. Drira, M. Jmaiel, Mining approach for software architectures’ description discovery, in: Proceedings of the 14th IEEE/ACS  International Conference on Computer Systems and Applications (AICCSA), 2017, pp. 879–886 \\
% {[S52]}	M. Nicoletti, J. A. Diaz-Pace, S. Schiaffino, Towards software architecture documents matching stakeholders’ interests, in: Proceedings of the 2nd International Conference on Advances in New Technologies, Interactive Interfaces, and Communicability (ADNTIIC), 2011, pp. 176–185 \\
% {[S53]}	J. Musil, F. J. Ekaputra, M. Sabou, T. Ionescu, D. Schall, A. Musil, S. Biffl, Continuous architectural knowledge integration: Making heterogeneous architectural knowledge available in large-scale organizations, in: Proceedings of the 14th IEEE International Conference on Software Architecture (ICSA), 2017, pp. 189–192 \\
% {[S54]}	R. Weinreich, G. Buchgeher, Towards supporting the software architecture life cycle, Journal of Systems and Software 85 (3) (2012) 546–561 \\
% {[S55]}	P. R. Anish, B. Balasubramaniam, J. Cleland-Huang, R. Wieringa, M. Daneva, S. Ghaisas, Identifying architecturally significant functional requirements, in: Proceedings of the 5th International Workshop on the Twin Peaks of Requirements and Architecture (TwinPeaks), 2015, pp. 3–8 \\
% {[S56]}	D. E. Krutz, M. Mirakhorl, Architectural clones: toward tactical code reuse, in: Proceedings of the 31st Annual ACM Symposium on Applied Computing (SAC), 2016, pp. 1480–1485 \\
% {[S57]}	M. Mirakhorli, J. Cleland-Huang, Detecting, tracing, and monitoring architectural tactics in code, IEEE Transactions on Software Engineering 42 (3) (2015) 205–220 \\
% {[S58]}	R. Duddukuri, T. Prabhakar, Helping architects in retrieving architecture documents: A semantic based approach, in: Proceedings of the 1st International Workshop on Semantic Matchmaking and Resource Retrieval (SMR), 2006, pp. 113-120 \\
% {[S59]}	L. do Nascimento Vale, M. d. A. Maia, Keecle: Mining key architecturally relevant classes using dynamic analysis, in: Proceedings of the 31st IEEE International Conference on Software Maintenance and Evolution (ICSME), 2015, pp. 566–570 \\
% {[S60]}	M. Nayrolles, F. Palma and N. Moha and Y. Gu{\'e}h{\'e}neuc, SODA: A Tool Support for the Detection of SOA Antipatterns, in: Proceedings of the 10th International Conference on Service-Oriented Computing (ICSOC), 2012, pp.451-455 \\
% {[S61]}	T. L. Babu, M. S. Ramaiah, T. Prabhakar, D. Rambabu, Archvoc–towards an ontology for software architecture, in: Proceedings of the 2nd Workshop on Sharing and Reusing Architectural Knowledge-Architecture, Rationale, and Design Intent (SHARK/ADI), 2007, pp. 5–10 \\
% {[S62]}	E. Maggiori, L. Gervasoni, M. Antúnez, A. Rago, and J. A. D\'{i}az-Pace, Towards recovering architectural information from images of architectural diagrams, in: Proceedings of the 15th Argentine Symposium on Software Engineering (ASSE), 2014, pp. 36–50 \\
% {[S63]}	D. Liu, Z.-L. Ren, Z.-T. Long, G.-J. Gao, H. Jiang, Mining design pattern use scenarios and related design pattern pairs: A case study on online posts, Journal of Computer Science and Technology 35 (5) (2020) 963–978 \\
% {[S64]}	R. Mo, Y. Cai, R. Kazman, L. Xiao, Q. Feng, Architecture anti-patterns: Automatically detectable violations of design principles, IEEE Transactions on Software Engineering 47 (5) (2019) 1008–1028 \\
% {[S65]} Pigazzini, Ilaria, Automatic Detection of Architectural Bad Smells through Semantic Representation of Code, In: Proceedings of the 13th European Conference on Software Architecture, (ECSA), 2019, pp.59-62 \\
% {[S66]}	G. Gokyer, S. Cetin, C. Sener, M. T. Yondem, Non-functional requirements to architectural concerns: {ML} and {NLP} at crossroads, in: Proceedings of the 3rd International Conference on Software Engineering Advances (ICSEA), 2008, pp. 400–406 \\
% {[S67]}	I. Sora, C. B. Chirila, Finding key classes in object-oriented software systems by techniques based on static analysis, Information and Software Technology 116 (2019) 106176 \\
% {[S68]}	B. S. Mitchell, S. Mancoridis, On the automatic modularization of software systems using the bunch tool, IEEE Transactions on Software Engineering 32 (3) (2006) 193–208 \\
% {[S69]}	Y. Zhang, R. Witte, J. Rilling, V. Haarslev, Ontology-based program comprehension tool supporting website architectural evolution, in: Proceedings of the 8th IEEE International Symposium on Web Site Evolution (WSE), 2006, pp. 41–49 \\
% {[S70]}	R. C. de Boer, Architectural knowledge discovery: Why and how?, ACM SIGSOFT Software Engineering Notes 31 (5) (2006) 1–4. \\
% {[S71]}	J. A. D\'{ı}az-Pace, A. Tommasel, D. Godoy, Towards anticipation of architectural smells using link prediction techniques, in: Proceedings of the 18th IEEE International Working Conference on Source Code Analysis and Manipulation (SCAM), 2018, pp. 62–71 \\
% {[S72]}	M. Nayrolles, N. Moha, P. Valtchev, Improving SOA antipatterns detection in service based systems by mining execution traces, in: Proceedings of the 20th Working Conference on Reverse Engineering (WCRE), 2013, pp. 321–330 \\
% {[S73]}	V. Bandara, I. Perera, Identifying software architecture erosion through code comments, in: Proceedings of the 18th International Conference on Advances in ICT for Emerging Regions (ICTer), 2018, pp. 62–69 \\
% {[S74]}	A. Zaidman, S. Demeyer, Automatic identification of key classes in a software system using web mining techniques, Journal of Software Maintenance and Evolution: Research and Practice 20 (6) (2008) 387–417 \\
% {[S75]}	S. Chardigny, A. Seriai, M. Oussalah, D. Tamzalit, Extraction of component-based architecture from object-oriented systems, in: Proceeding of the 7th working IEEE/IFIP Conference on Software Architecture (WICSA), 2008, pp. 285–288 \\
% {[S76]}	M. Lu, P. Liang, Automatic classification of non-functional requirements from augmented app user reviews, in: Proceedings of the 21st International Conference on Evaluation and Assessment in Software Engineering (EASE), 2017, pp. 344–353 \\
% {[S77]}	A. K. Mondal, C. K. Roy, K. A. Schneider, B. Roy, S. S. Nath, Semantic slicing of architectural change commits: Towards semantic design review, in: Proceedings of the 15th ACM/IEEE International Symposium on Empirical Software Engineering and Measurement (ESEM), 2021, pp. 1–6 \\
% {[S78]} A. W. Kamal, P. Avgeriou, Mining relationships between the participants of architectural patterns, in: Proceedings of the 4th European Conference on Software Architecture (ECSA), 2010, pp. 401–408 \\
% {[S79]}	M. Ali, H. Mushtaq, M. B. Rasheed, A. Baqir, T. Alquthami, Mining software architecture knowledge: Classifying stack overflow posts using machine learning, Concurrency and Computation: Practice and Experience 33 (16) (2021) e6277 \\
% {[S80]}	C. Timperley,  S Bradley, T. D{\"u}rschmid, D. Schmerl, C. Garlan, Le Goues, ROSDiscover: Statically Detecting Run-Time Architecture Misconfigurations in Robotics Systems, in: Proceedings of the 19th International Conference on Software Architecture (ICSA), 2022, pp. 112--123 \\
% {[S81]} A. Landi, D. San Mart{\'\i}n, B. Santos, R. W. Cunha, V. Camargo, Architectural conformance checking for KDM-represented systems, Journal of Systems and Software 183 (2022) 111116 \\
% {[S82]} D. Liu, H. Jiang, X. Li, Z. Ren, L. Qiao, Z. Ding, DPWord2Vec: better representation of design patterns in semantics, IEEE Transactions on Software Engineering 48 (4) (2022) 1228--1248 \\
% {[S83]} G. Rodriguez, J. D{\'\i}az-Pace, L. Berdun, S. Misra, Deriving Architectural Responsibilities from Textual Requirements, in: Proceedings of the 1st International Conference on Informatics and Intelligent Applications (ICIIA), 2021, pp. 297--310 \\
% {[S84]} D. Dobrean, L. Dio{\c{s}}an, Pathways for statically mining the Model-View-Controller software architecture on mobile applications, Soft Computing 26 (19) (2022) 10493--10511\\
% {[S85]} A. Singjai, U. Zdun, API Description-Based Conformance Assessment of Architectural Design Decision, in: Proceedings of the 16th IEEE International Conference on Service-Oriented System Engineering (SOSE), 2022, pp. 59--68 \\
% {[S86]} A. Singjai, U. Zdun, Conformance Assessment of Architectural Design Decisions on the Mapping of Domain Model Elements to APIs and API Endpoints, in: Proceedings of the 19th IEEE International Conference on Software Architecture Companion (ICSA-C), 2022, pp. 76--83 \\
% {[S87]} L. Wijerathna, A. Aleti, T. Bi, A. Tang, Mining and relating design contexts and design patterns from Stack Overflow, Empirical Software Engineering 27 (8) (2022)  \\
% {[S88]} D. Sas, P. Avgeriou, U. Uyumaz, On the evolution and impact of architectural smells—an industrial case study, Empirical Software Engineering 27 (86) (2022) \\
% {[S89]} F. A. Fontana, Francesca, I. Pigazzini, R. Roveda, M. Zanoni, Automatic detection of instability architectural smells, in: Proceedings of the 32nd IEEE International Conference on Software Maintenance and Evolution (ICSME), 2016, pp. 433--437 \\
% {[S90]} A. Biaggi, F. A. Fontana, R. Roveda , An architectural smells detection tool for c and c++ projects, in: Proceedings of the 44th Euromicro Conference on Software Engineering and Advanced Applications (SEAA), 2018, pp. 417--420 \\
% {[S91]} D. M. Leand, D. Link, A. Shahbazian, N. Medvidovic, An Empirical Study of Architectural Decay in Open-Source Software, in: Proceedings of the 15th IEEE International Conference on Software Architecture (ICSA), 2018, pp. 176--185 \\
% {[S92]} A. Martini, F. A. Fontana, A. Andrea, R. Roveda, Identifying and prioritizing architectural debt through architectural smells: a case study in a large software company, in: Proceedings of the 12th European Conference on Software Architecture (ECSA), 2018, pp. 320--335 \\
% {[S93]} R. Mo, Y. Cai, R. Kazman, L. Xiao, Hotspot patterns: The formal definition and automatic detection of architecture smells, in: Proceedings of the 12th Working IEEE/IFIP Conference on Software Architecture (WICSA), 2015, pp. 51--60 \\
% {[S94]} R. Mo, W. Snipes, Y. Cai, S. Ramaswamy, R. Kazman, M. Naedele , Experiences applying automated architecture analysis tool suites, in: Proceedings of the 33rd ACM/IEEE International Conference on Automated Software Engineering (ASE), 2018, pp. 779--789 \\
% {[S95]} Q. Feng, Y. Cai, R. Kazman, D. Cui, T. Liu, H. Fang, Active hotspot: An issue-oriented model to monitor software evolution and degradation, in: Proceedings of the 34th IEEE/ACM International Conference on Automated Software Engineering (ASE), 2019, pp. 986--997 \\
% {[S96]} M. Nayebi, Y. Cai, R. Kazman, G. Ruhe, Q. Feng, C. Carlson, F. Chew, A longitudinal study of identifying and paying down architecture debt, in: Proceedings of the 41st IEEE/ACM International Conference on Software Engineering: Software Engineering in Practice (ICSE-SEIP), 2019, pp. 171--180 \\
% {[S97]} D. Sas, P. Avgeriou, F. A. Fontana, Investigating instability architectural smells evolution: an exploratory case study, in: Proceedings of the 35th IEEE International Conference on Software Maintenance and Evolution (ICSME), 2019, pp. 557--567 \\  
% {[S98]} D. M. Le, C. Carrillo, R. Capilla, N. Medvidovic, Relating architectural decay and sustainability of software systems, in: Proceedings of the 13th Working IEEE/IFIP Conference on Software Architecture (WICSA), 2016, pp. 178--181 \\
% {[S99]} F. A. Fontana, I. Pigazzini, R. Roveda, D. Tamburri, M. Zanoni, N. Di, Arcan: A tool for architectural smells detection, in: Proceedings of the 3rd IEEE International Conference on Software Architecture Workshops (ICSAW), 2017, pp. 282--285 \\
% {[S100]} P. Velasco-Elizondo, L. Casta{\~n}eda-Calvillo, A. Garc{\'\i}a-Fernandez, S. Vazquez-Reyes, Towards detecting MVC architectural smells, in: Proceedings of the 6th International Conference on Software Process Improvement (CIMPS), 2018, pp. 251--260 \\
% {[S101]} Y. Cai, H. Wang, S. Wong, L. Wang, Leveraging design rules to improve software architecture recovery, in: Proceedings of the 9th International ACM SIGSOFT Conference on Quality of Software Architectures (QoSA), 2013, pp. 133--142 \\
% {[S102]} D. Link, P. Behnamghader, R. Moazeni, B. Boehm, Recover and RELAX: Concern-oriented software architecture recovery for systems development and maintenance, in: Proceedings of the 23rd IEEE/ACM International Conference on Software and System Processes (ICSSP), 2019, pp. 64--73 \\
% {[S103]} D. Dobrean, L. Dio{\c{s}}an, On What Kind of Applications Can Clustering Be Used for Inferring MVC Architectural Layers? in: Proceedings of the 30th International Conference on Information Systems Development (ISD), 2022, pp. 115--131 \\
% {[S104]} A. Zakurdaeva, M. Weiss, S. Muegge, Detecting architectural integrity violation patterns using machine learning, in: Proceedings of the 35th Annual ACM Symposium on Applied Computing (SAC), 2020, pp. 1480--1487 \\

% \subsection*{Appendix B. Distribution of the Selected Studies in Publication Venues}\label{SelectedStudiesInVenues}

% \small
% \begin{longtable}{p{0cm}p{8.2cm}p{1.5cm}p{0.1cm}}
% \caption{Distribution of the selected studies in publication venues} \label{PublicationVenues} \\
% \hline \multicolumn{1}{l} {\textbf{\#}} & \multicolumn{1}{l}{\textbf{Publication venue}} & \multicolumn{1}{l}{\textbf{Type}} & \multicolumn{1}{l}{\textbf{No.}}\\ \hline 
% \endfirsthead
% \multicolumn{4}{l}%
% {{\bfseries }}\\ 
% \endhead
% \multicolumn{4}{r}{{}} \\ 
% \endfoot
% \hline
% \endlastfoot
%     1   & International Conference on Software Architecture (ICSA)                                                          & Conference  & 10\\
%     2   & European Conference on Software Architecture (ECSA)                                                               & Conference  & 7\\
%     3   & Journal of Systems and Software                                                                                   & Journal     & 6\\
%     4   & IEEE Transactions on Software Engineering                                                                         & Journal     & 5\\
%     5   & International Conference of Software Engineering (ICSE)                                                           & Conference  & 5\\
%     6   & Empirical Software Engineering                                                                                    & Journal     & 4\\
%     7   & Information and Software Technology                                                                               & Journal     & 3\\
%     8   & International Conference on software maintenance and evolution (ICSME)                                            & Conference  & 3\\
%     9   & International Conference on Automated Software Engineering (ASE)                                                  & Conference  & 3\\
%    10   & Science of Computer Programming                                                                                   & Journal     & 2\\ 
%    11   & International Conference on Evaluation and Assessment in Software Engineering (EASE)                              & Conference  & 2\\ 
%    12   & International Working Conference on Mining Software Repositories (MSR)                                            & Conference  & 2\\
%    13   & International Conference on Software Engineering and Knowledge Engineering (SEKE)                                 & Conference  & 2\\
%    14   & International Conference on Software Architecture Workshops (ICSAW)                                               & Workshop    & 3\\
%    15   & Workshop on Sharing and Reusing Architectural Knowledge (SHARK)                                                   & Workshop    & 2\\   
% \end{longtable}
% \normalsize

%////////////////////////////////////////////////////////////////////////////////////////////////////////////////////////////////////////////////////////

% \subsection*{Appendix C. Abbreviation used in this SMS}

% \small
% \begin{longtable}{p{8em}p{26em}}
% \caption{Abbreviations used in this SMS} \label{Abbreviation} \\
% \hline \multicolumn{1}{l} {\textbf{Abbreviation}} & \multicolumn{1}{l}{\textbf{Full name}}\\ \hline 
% \endfirsthead

% \multicolumn{2}{l}%
% {{\bfseries }}\\ 
% \endhead
% %\hline 
% \multicolumn{2}{r}{{}} \\ 
% \endfoot

% \hline
% \endlastfoot
%                                     AA       & Architecture Analysis\\
%                                     AST      & Abstract Syntax Tree\\
%                                     ACC      & Architecture Conformance Checking\\
%                                     ADp      & Architectural Description and Documentation\\ 
%                                     AE       & Architecture Evaluation\\
%                                     AIm       & Architecture Implementation\\
%                                     AIA      & Architecture Impact Analysis\\
%                                     AK       & Architecture Knowledge\\
%                                     AME      & Architecture Maintenance and Evolution\\
%                                     ARec     & Architecture Recovery\\
%                                     AReu     & Architecture Reuse\\
%                                     AS       & Architecture Synthesis\\
%                                     ASR      & Architecturally Significant Requirement\\
%                                     AT       & Architectural Tactic\\
%                                     ATD      & Architectural Technical Debt\\
%                                     AU       & Architecture Understanding\\
%                                     DL       & Deep Learning\\
%                                     LDA      & Latent Dirichlet Allocation\\
%                                     LP       & Link Prediction\\
%                                     MDG      & Module Dependency Graph\\
%                                     ML       & Machine Learning\\
%                                     MSR      & Mining Software Repositories\\
%                                     MaRK     & Mining Requirements Knowledge\\
%                                     NLP4RE   & Natural Language Processing for Requirements Engineering\\
%                                     NFR      & Non-Functional Requirement\\
%                                     NLP      & Natural Language Processing\\
%                                     OSS      & Open Source Software\\
%                                     POS      & Part of Speech\\
%                                     QA       & Quality Attribute\\
%                                     Q\&A     & Question and Answers\\
%                                     RQ       & Research Question\\
%                                     SA       & Software Architecture\\
%                                     SMS      & Systematic Mapping Study\\
%                                     SLR      & Systematic Literature Review\\
%                                     VCS      & Version Control Systems\\
                                    
% \end{longtable}
%\normalsize




%//////////////////////////////////////////////////////////////////////////////////////////////////////////////
%\section*{Data Availability Statements} \label{dataavailability}
%The data of this work will be made available on reasonable request.
